# Supplementary material for: Pre- and post-processing of cluster galaxies out to $5 \times R_{200}$: The extreme case of A2670
Source: arXiv:2401.06973 source file (2024-01-13)
Supplement: Supplementary file 1 [file supplement_extra_figs.pdf]

### Supplementary material 1: Atlas of RPS Candidates

Legacy Survey RGB composite images for all the ram-pressure stripped "jellyfish" (JF) candidates in A2670 split by clustercentric distances ($r$). Figure 1 displays JF candidates inside the cluster ($r < 2.5 \times R_{200}$) and Figure 2 those in the outskirts (between 2.5 and $5 \times R_{200}$). Galaxy ID and vote fraction ($F_{\mathrm{RPS}}$ are labeled in each case). Only cases with $F_{\mathrm{RPS}} > 0.5$ were considered.

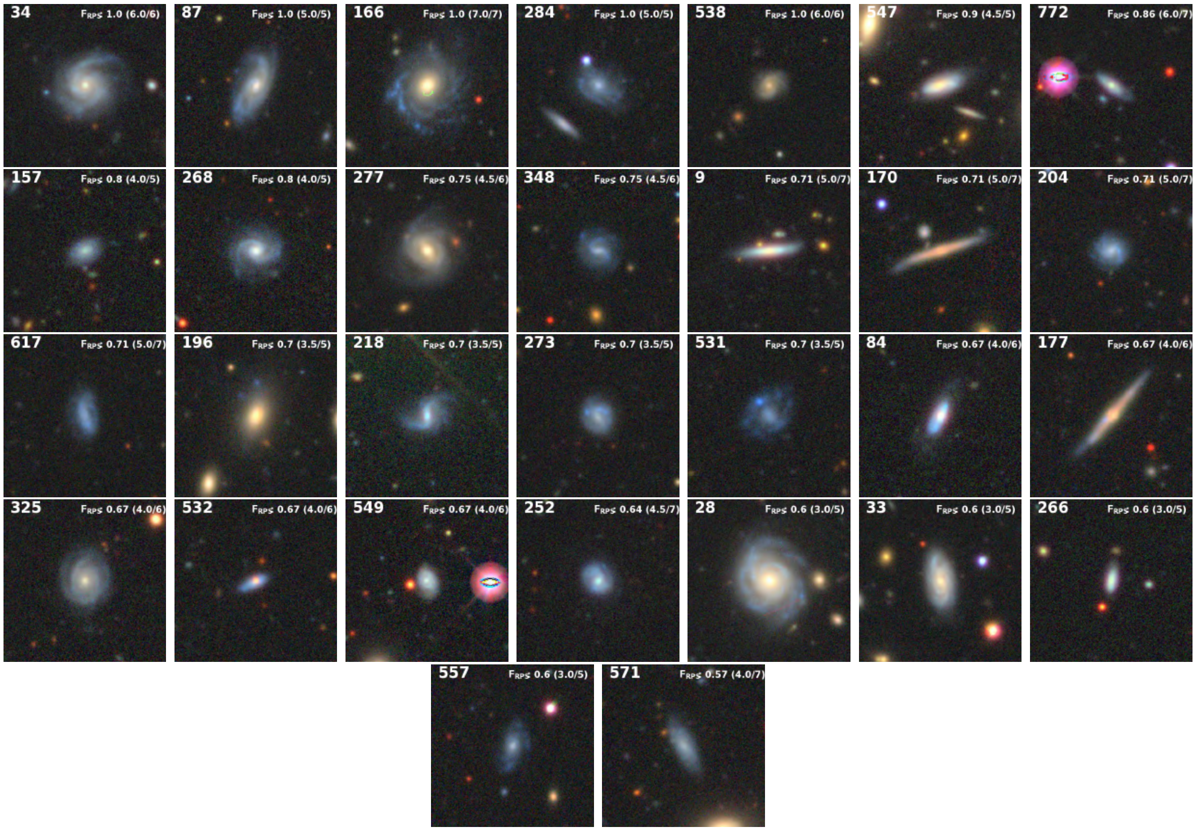


Figure 1: Examples of JF galaxies with high RPS vote fractions located less than $2.5 \times R_{200}$, sorted from high to low $F_{RPS}$ values.

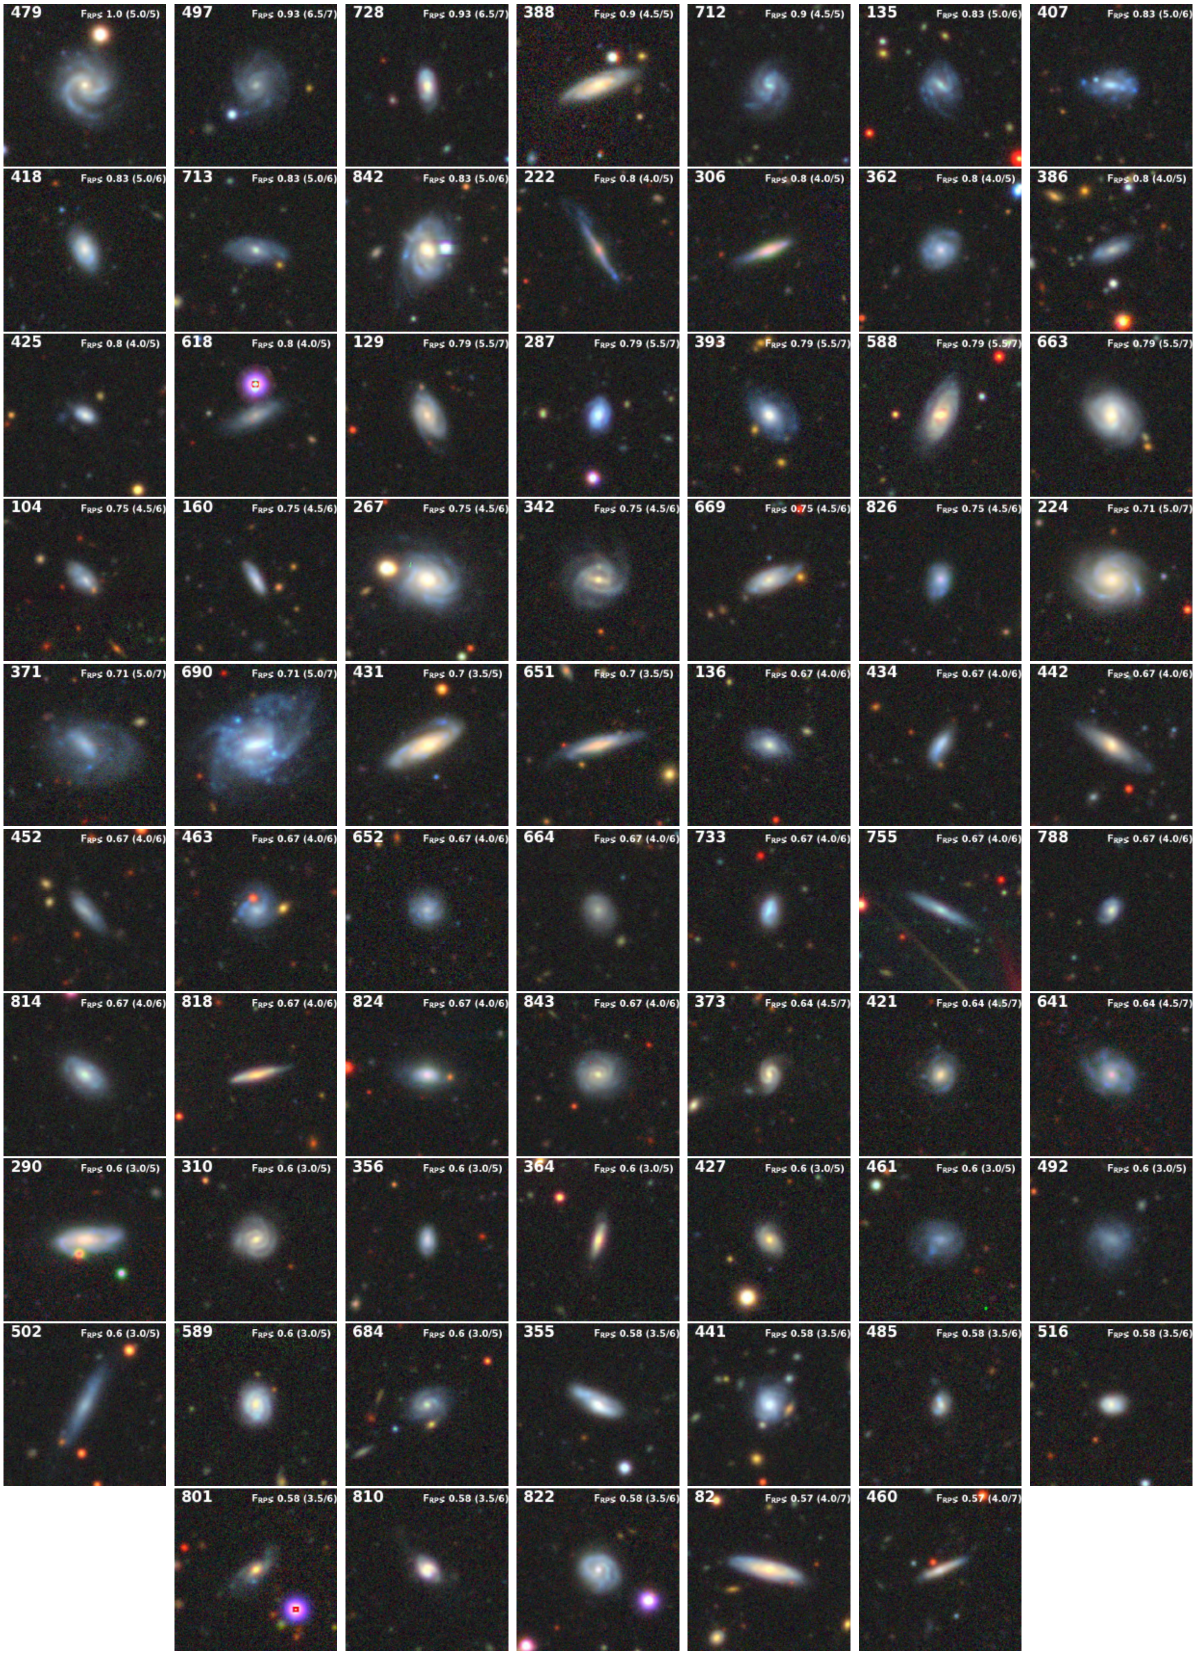


Figure 2: Examples of JF galaxies with high RPS vote fractions located between 2.5 and $5 \times R_{200}$, sorted from high to low $F_{RPS}$ values. Note that some of these are bound to the cluster (e.g. ID: 842, 843) but not all. For example, galaxies with ID: 135, 222, 712 are JF candidates with high $F_{RPS}$, located in the eastern sheet out in the cluster outskirts at $> 4 \times R_{200}$.
