# Supplementary material for: Pre- and post-processing of cluster galaxies out to $5 \times R_{200}$: The extreme case of A2670
Source: arXiv:2401.06973 source file (2024-01-13)
Supplement: Supplementary file 2 [file supplement_full_table.pdf]

## Supplementary material 2: Table of disturbed galaxies

Table 1: The first column of the table indicates the ID of the galaxies in our catalogue. The second and third column contain the coordinates of the galaxies in degrees, R.A. and Dec., respectively. The fourth column contains the final category assigned to the galaxy using the different votes of each classifier. The fifth, sixth and seventh column contain the vote fraction for each class, $F_{\mathrm{RPS}}$, $F_{\mathrm{GRAV}}$ and $F_{\mathrm{N.I.}}$, respectively.

| ID | R.A. | Dec. | Final Category | $F_{\mathrm{RPS}}$ | $F_{\mathrm{GRAV}}$ | $F_{\mathrm{N.I.}}$ |
|---|---|---|---|---|---|---|
| 7 | 358.49480 | -10.69413 | M | 0.100 | 0.500 | 0.400 |
| 9 | 358.53481 | -10.57998 | JF | 0.714 | 0.143 | 0.143 |
| 13 | 358.49525 | -10.69191 | JM | 0.300 | 0.700 | 0.000 |
| 28 | 358.72571 | -10.28808 | JF | 0.600 | 0.000 | 0.400 |
| 30 | 358.69096 | -10.24600 | JM | 0.700 | 0.300 | 0.000 |
| 33 | 359.08307 | -10.21275 | JF | 0.600 | 0.000 | 0.400 |
| 34 | 358.26567 | -11.08203 | JF | 1.000 | 0.000 | 0.000 |
| 35 | 357.02268 | -10.71181 | JF | 0.500 | 0.000 | 0.500 |
| 40 | 358.04252 | -10.30951 | M | 0.000 | 0.714 | 0.286 |
| 43 | 359.01519 | -11.18858 | JF | 0.500 | 0.500 | 0.000 |
| 52 | 358.50602 | -10.21325 | PM | 0.000 | 0.600 | 0.400 |
| 67 | 358.53431 | -10.20781 | M | 0.000 | 0.500 | 0.500 |
| 76 | 358.54199 | -10.40703 | M | 0.000 | 0.500 | 0.500 |
| 82 | 357.54160 | -9.04424 | JF | 0.571 | 0.000 | 0.429 |
| 83 | 359.82906 | -9.33143 | PM | 0.000 | 1.000 | 0.000 |
| 84 | 358.66306 | -11.17487 | JF | 0.667 | 0.333 | 0.000 |
| 87 | 358.68413 | -10.28220 | JF | 1.000 | 0.000 | 0.000 |
| 104 | 358.15778 | -8.94071 | JF | 0.750 | 0.250 | 0.000 |
| 105 | 358.81385 | -10.97464 | M | 0.300 | 0.700 | 0.000 |
| 110 | 358.55513 | -10.38638 | M | 0.071 | 0.929 | 0.000 |
| 119 | 359.22704 | -10.26874 | M | 0.000 | 0.833 | 0.167 |
| 124 | 357.57138 | -10.19963 | M | 0.000 | 0.600 | 0.400 |
| 125 | 358.77058 | -10.35581 | PM | 0.143 | 0.714 | 0.143 |
| 127 | 359.11609 | -9.30547 | JM | 0.500 | 0.333 | 0.167 |
| 129 | 358.99402 | -9.50826 | JF | 0.786 | 0.214 | 0.000 |
| 131 | 359.22668 | -10.26791 | M | 0.000 | 0.714 | 0.286 |
| 133 | 358.48580 | -10.25292 | M | 0.143 | 0.857 | 0.000 |
| 134 | 358.53200 | -10.01322 | PM | 0.000 | 1.000 | 0.000 |
| 135 | 359.82718 | -10.64715 | JF | 0.833 | 0.167 | 0.000 |
| 136 | 357.40130 | -8.94153 | JF | 0.667 | 0.000 | 0.333 |
| 137 | 358.72339 | -10.32546 | JM | 0.500 | 0.167 | 0.333 |
| 140 | 358.17773 | -9.77037 | JF | 0.500 | 0.000 | 0.500 |
| 145 | 358.35993 | -10.26360 | JF | 0.500 | 0.000 | 0.500 |
| 157 | 358.53183 | -10.89376 | JF | 0.800 | 0.000 | 0.200 |
| 160 | 358.19361 | -9.39617 | JF | 0.750 | 0.083 | 0.167 |
| 164 | 358.91854 | -9.55243 | M | 0.000 | 0.667 | 0.333 |
| 166 | 358.65902 | -10.31880 | JF | 1.000 | 0.000 | 0.000 |
| 168 | 359.16952 | -10.81769 | JM | 0.100 | 0.500 | 0.400 |
| 170 | 358.25328 | -9.57316 | JF | 0.714 | 0.143 | 0.143 |
| 171 | 358.62848 | -10.22337 | PM | 0.000 | 0.857 | 0.143 |
| 174 | 358.25881 | -10.92653 | PM | 0.417 | 0.583 | 0.000 |
| 177 | 358.57615 | -10.23046 | JF | 0.667 | 0.000 | 0.333 |
| 179 | 358.97778 | -9.22967 | PM | 0.300 | 0.500 | 0.200 |
| 186 | 358.18622 | -10.29496 | PM | 0.000 | 0.500 | 0.500 |

**Table 1 continued from previous page**

| | | | | | | |
|---|---|---|---|---|---|---|
| 190 | 357.49733 | -9.79894 | JF | 0.500 | 0.000 | 0.500 |
| 194 | 358.95637 | -9.39853 | M | 0.000 | 0.500 | 0.500 |
| 195 | 358.41611 | -10.42991 | JM | 0.400 | 0.600 | 0.000 |
| 196 | 358.57647 | -10.33747 | JF | 0.700 | 0.100 | 0.200 |
| 198 | 358.52930 | -10.42132 | M | 0.000 | 0.500 | 0.500 |
| 204 | 358.35536 | -10.04006 | JF | 0.714 | 0.000 | 0.286 |
| 211 | 358.76653 | -10.51664 | PM | 0.000 | 0.800 | 0.200 |
| 217 | 357.57541 | -10.19743 | M | 0.200 | 0.400 | 0.400 |
| 218 | 358.29533 | -11.03420 | JF | 0.700 | 0.300 | 0.000 |
| 222 | 359.93771 | -9.53557 | JF | 0.800 | 0.200 | 0.000 |
| 224 | 359.87962 | -9.91379 | JF | 0.714 | 0.000 | 0.286 |
| 227 | 358.48842 | -10.38032 | M | 0.000 | 0.800 | 0.200 |
| 234 | 358.49079 | -9.10317 | JM | 0.250 | 0.417 | 0.333 |
| 236 | 357.23466 | -9.06688 | JF | 0.400 | 0.200 | 0.400 |
| 239 | 358.81129 | -10.49654 | M | 0.000 | 0.667 | 0.333 |
| 243 | 358.19735 | -10.88310 | PM | 0.000 | 0.833 | 0.167 |
| 252 | 358.68154 | -10.93081 | JF | 0.643 | 0.214 | 0.143 |
| 260 | 358.44444 | -10.27081 | JF | 0.429 | 0.143 | 0.429 |
| 263 | 358.65125 | -9.02668 | M | 0.286 | 0.571 | 0.143 |
| 266 | 359.36878 | -10.45888 | JF | 0.600 | 0.200 | 0.200 |
| 267 | 356.84795 | -10.78096 | JF | 0.750 | 0.250 | 0.000 |
| 268 | 358.84038 | -9.60657 | JF | 0.800 | 0.000 | 0.200 |
| 273 | 358.36167 | -10.41159 | JF | 0.700 | 0.100 | 0.200 |
| 277 | 358.32949 | -10.38424 | JF | 0.750 | 0.083 | 0.167 |
| 283 | 358.74814 | -9.24707 | M | 0.000 | 1.000 | 0.000 |
| 284 | 358.64907 | -9.96356 | JF | 1.000 | 0.000 | 0.000 |
| 285 | 358.58131 | -10.55010 | JF | 0.417 | 0.250 | 0.333 |
| 286 | 357.41333 | -10.00713 | M | 0.000 | 0.600 | 0.400 |
| 287 | 359.48998 | -10.53390 | JF | 0.786 | 0.071 | 0.143 |
| 290 | 359.91075 | -9.55799 | JF | 0.600 | 0.000 | 0.400 |
| 291 | 357.96055 | -10.38551 | JM | 0.200 | 0.400 | 0.400 |
| 293 | 358.81121 | -9.13957 | M | 0.083 | 0.917 | 0.000 |
| 296 | 358.57536 | -10.41544 | M | 0.000 | 0.600 | 0.400 |
| 297 | 359.16884 | -9.11901 | M | 0.250 | 0.417 | 0.333 |
| 304 | 359.99483 | -9.69295 | JF | 0.400 | 0.200 | 0.400 |
| 305 | 357.75500 | -10.01107 | M | 0.100 | 0.900 | 0.000 |
| 306 | 359.65528 | -9.31968 | JF | 0.800 | 0.000 | 0.200 |
| 310 | 358.31430 | -8.78573 | JF | 0.600 | 0.000 | 0.400 |
| 320 | 357.58919 | -8.88501 | M | 0.000 | 1.000 | 0.000 |
| 325 | 357.74023 | -10.55045 | JF | 0.667 | 0.333 | 0.000 |
| 330 | 357.09422 | -9.53560 | JF | 0.400 | 0.400 | 0.200 |
| 340 | 359.50640 | -9.22128 | JM | 0.333 | 0.333 | 0.333 |
| 342 | 357.22353 | -8.85431 | JF | 0.750 | 0.083 | 0.167 |
| 348 | 357.85426 | -9.95125 | JF | 0.750 | 0.250 | 0.000 |
| 355 | 357.61752 | -10.43200 | JF | 0.583 | 0.417 | 0.000 |
| 356 | 359.41487 | -8.72869 | JF | 0.600 | 0.000 | 0.400 |
| 358 | 358.27844 | -8.79123 | JF | 0.429 | 0.286 | 0.286 |
| 362 | 359.99389 | -8.72214 | JF | 0.800 | 0.200 | 0.000 |
| 364 | 357.75039 | -8.84456 | JF | 0.600 | 0.000 | 0.400 |
| 371 | 356.80080 | -12.06758 | JF | 0.714 | 0.143 | 0.143 |
| 373 | 356.86549 | -11.97720 | JF | 0.643 | 0.357 | 0.000 |
| 383 | 357.06170 | -12.05838 | PM | 0.143 | 0.714 | 0.143 |
| 384 | 357.05070 | -12.04698 | M | 0.357 | 0.643 | 0.000 |

**Table 1 continued from previous page**

| | | | | | | |
|---|---|---|---|---|---|---|
| 386 | 357.03676 | -11.98044 | JF | 0.800 | 0.000 | 0.200 |
| 388 | 357.10855 | -12.06815 | JF | 0.900 | 0.100 | 0.000 |
| 393 | 356.77461 | -11.63899 | JF | 0.786 | 0.071 | 0.143 |
| 403 | 357.10259 | -11.83976 | JM | 0.200 | 0.600 | 0.200 |
| 406 | 357.26481 | -11.87509 | M | 0.000 | 0.500 | 0.500 |
| 407 | 357.09747 | -11.75161 | JF | 0.833 | 0.167 | 0.000 |
| 417 | 357.33292 | -12.12778 | M | 0.200 | 0.800 | 0.000 |
| 418 | 357.61599 | -12.19887 | JF | 0.833 | 0.000 | 0.167 |
| 419 | 357.58502 | -12.12266 | M | 0.143 | 0.857 | 0.000 |
| 420 | 357.58596 | -12.12182 | M | 0.071 | 0.929 | 0.000 |
| 421 | 357.69533 | -12.18937 | JF | 0.643 | 0.071 | 0.286 |
| 425 | 357.83868 | -11.97430 | JF | 0.800 | 0.200 | 0.000 |
| 427 | 358.06661 | -12.08680 | JF | 0.600 | 0.000 | 0.400 |
| 429 | 357.44842 | -11.81442 | JM | 0.200 | 0.800 | 0.000 |
| 431 | 357.67743 | -11.88525 | JF | 0.700 | 0.100 | 0.200 |
| 432 | 357.69505 | -11.88823 | JF | 0.500 | 0.333 | 0.167 |
| 434 | 357.54904 | -11.65835 | JF | 0.667 | 0.167 | 0.167 |
| 436 | 357.84524 | -11.81301 | JF | 0.333 | 0.333 | 0.333 |
| 441 | 357.99959 | -11.78091 | JF | 0.583 | 0.083 | 0.333 |
| 442 | 357.86771 | -11.57126 | JF | 0.667 | 0.000 | 0.333 |
| 443 | 357.85516 | -11.56616 | JF | 0.417 | 0.250 | 0.333 |
| 446 | 358.05106 | -11.67363 | M | 0.000 | 1.000 | 0.000 |
| 447 | 358.05252 | -11.67492 | M | 0.000 | 1.000 | 0.000 |
| 449 | 357.99896 | -11.50903 | PM | 0.000 | 1.000 | 0.000 |
| 452 | 356.77531 | -11.13127 | JF | 0.667 | 0.000 | 0.333 |
| 459 | 356.94682 | -11.11188 | M | 0.000 | 1.000 | 0.000 |
| 460 | 357.29145 | -11.20970 | JF | 0.571 | 0.000 | 0.429 |
| 461 | 356.76275 | -10.73378 | JF | 0.600 | 0.200 | 0.200 |
| 463 | 357.48648 | -11.46494 | JF | 0.667 | 0.333 | 0.000 |
| 470 | 357.90925 | -11.45150 | M | 0.000 | 1.000 | 0.000 |
| 475 | 358.16944 | -11.39817 | JM | 0.357 | 0.357 | 0.286 |
| 478 | 357.99938 | -11.26975 | M | 0.000 | 1.000 | 0.000 |
| 479 | 357.84451 | -11.12915 | JF | 1.000 | 0.000 | 0.000 |
| 480 | 358.16680 | -11.20586 | M | 0.000 | 0.833 | 0.167 |
| 481 | 358.17155 | -11.20496 | M | 0.000 | 1.000 | 0.000 |
| 482 | 358.09223 | -11.07317 | M | 0.083 | 0.750 | 0.167 |
| 485 | 357.49332 | -10.82193 | JF | 0.583 | 0.417 | 0.000 |
| 492 | 358.49303 | -12.16549 | JF | 0.600 | 0.000 | 0.400 |
| 497 | 358.38001 | -11.92804 | JF | 0.929 | 0.071 | 0.000 |
| 500 | 358.32702 | -11.83154 | PM | 0.000 | 0.667 | 0.333 |
| 502 | 358.28778 | -11.70974 | JF | 0.600 | 0.000 | 0.400 |
| 504 | 358.35676 | -11.73267 | JM | 0.333 | 0.333 | 0.333 |
| 505 | 358.47072 | -11.85894 | M | 0.200 | 0.800 | 0.000 |
| 507 | 358.39167 | -11.50539 | JF | 0.500 | 0.000 | 0.500 |
| 510 | 358.49953 | -11.66317 | PM | 0.000 | 0.500 | 0.500 |
| 512 | 358.29031 | -11.34935 | JM | 0.667 | 0.333 | 0.000 |
| 516 | 358.36276 | -11.33369 | JF | 0.583 | 0.083 | 0.333 |
| 523 | 358.25229 | -11.17124 | JF | 0.417 | 0.250 | 0.333 |
| 531 | 357.71679 | -10.46376 | JF | 0.700 | 0.300 | 0.000 |
| 532 | 358.13805 | -10.61129 | JF | 0.667 | 0.000 | 0.333 |
| 535 | 358.34444 | -10.54271 | M | 0.200 | 0.800 | 0.000 |
| 538 | 358.33703 | -10.44327 | JF | 1.000 | 0.000 | 0.000 |
| 543 | 358.51219 | -10.46514 | M | 0.167 | 0.500 | 0.333 |

**Table 1 continued from previous page**

| | | | | | | |
|---|---|---|---|---|---|---|
| 545 | 358.50879 | -10.43303 | M | 0.167 | 0.833 | 0.000 |
| 547 | 358.51908 | -10.43059 | JF | 0.900 | 0.100 | 0.000 |
| 549 | 358.55655 | -10.46340 | JF | 0.667 | 0.167 | 0.167 |
| 550 | 356.93242 | -10.10521 | M | 0.000 | 1.000 | 0.000 |
| 557 | 358.04979 | -9.86956 | JF | 0.600 | 0.400 | 0.000 |
| 560 | 357.18881 | -9.23955 | JF | 0.500 | 0.167 | 0.333 |
| 561 | 357.08640 | -9.07355 | JM | 0.643 | 0.214 | 0.143 |
| 564 | 357.99824 | -9.54075 | M | 0.083 | 0.917 | 0.000 |
| 565 | 357.58651 | -8.88589 | M | 0.000 | 1.000 | 0.000 |
| 566 | 357.76805 | -9.21759 | PM | 0.000 | 0.667 | 0.333 |
| 568 | 358.54689 | -10.40815 | M | 0.000 | 0.500 | 0.500 |
| 569 | 358.48798 | -10.37459 | M | 0.083 | 0.917 | 0.000 |
| 571 | 358.52008 | -10.32499 | JF | 0.571 | 0.000 | 0.429 |
| 572 | 358.55698 | -10.39026 | M | 0.000 | 1.000 | 0.000 |
| 573 | 358.55625 | -10.38574 | M | 0.100 | 0.900 | 0.000 |
| 575 | 358.48920 | -10.25349 | M | 0.000 | 1.000 | 0.000 |
| 583 | 358.49678 | -9.19279 | M | 0.000 | 0.600 | 0.400 |
| 588 | 357.59436 | -8.64785 | JF | 0.786 | 0.071 | 0.143 |
| 589 | 357.82511 | -8.62681 | JF | 0.600 | 0.000 | 0.400 |
| 592 | 358.57147 | -10.41568 | M | 0.000 | 0.800 | 0.200 |
| 593 | 358.56183 | -10.41358 | M | 0.250 | 0.750 | 0.000 |
| 595 | 358.60823 | -10.41115 | M | 0.000 | 0.667 | 0.333 |
| 597 | 358.55711 | -10.37252 | M | 0.000 | 0.500 | 0.500 |
| 612 | 358.89801 | -9.76580 | M | 0.333 | 0.667 | 0.000 |
| 617 | 359.13513 | -9.75631 | JF | 0.714 | 0.143 | 0.143 |
| 618 | 359.93535 | -10.12369 | JF | 0.800 | 0.000 | 0.200 |
| 626 | 358.95113 | -9.38944 | M | 0.100 | 0.900 | 0.000 |
| 629 | 358.74878 | -9.24803 | M | 0.000 | 0.833 | 0.167 |
| 630 | 358.74820 | -9.24562 | M | 0.000 | 1.000 | 0.000 |
| 636 | 358.69484 | -9.01189 | JF | 0.333 | 0.333 | 0.333 |
| 637 | 358.80014 | -9.06530 | JF | 0.500 | 0.000 | 0.500 |
| 641 | 359.84268 | -9.61400 | JF | 0.643 | 0.357 | 0.000 |
| 642 | 359.32888 | -9.16648 | PM | 0.000 | 0.500 | 0.500 |
| 645 | 359.99299 | -9.10078 | PM | 0.167 | 0.833 | 0.000 |
| 646 | 359.05929 | -8.86970 | PM | 0.200 | 0.600 | 0.200 |
| 647 | 358.70143 | -8.62838 | JM | 0.429 | 0.429 | 0.143 |
| 648 | 358.72309 | -8.61664 | M | 0.429 | 0.571 | 0.000 |
| 651 | 359.33505 | -8.65009 | JF | 0.700 | 0.100 | 0.200 |
| 652 | 359.64157 | -8.69734 | JF | 0.667 | 0.000 | 0.333 |
| 653 | 359.67563 | -8.64929 | JM | 0.500 | 0.333 | 0.167 |
| 662 | 358.98633 | -12.10047 | JF | 0.500 | 0.167 | 0.333 |
| 663 | 358.95031 | -12.04422 | JF | 0.786 | 0.214 | 0.000 |
| 664 | 358.57496 | -11.58301 | JF | 0.667 | 0.000 | 0.333 |
| 666 | 358.76102 | -11.70125 | JM | 0.357 | 0.357 | 0.286 |
| 668 | 358.68797 | -11.59825 | JF | 0.429 | 0.143 | 0.429 |
| 669 | 358.68007 | -11.57605 | JF | 0.750 | 0.250 | 0.000 |
| 677 | 359.51031 | -12.22012 | JM | 0.400 | 0.600 | 0.000 |
| 684 | 359.33770 | -12.02748 | JF | 0.600 | 0.000 | 0.400 |
| 690 | 359.50302 | -11.91512 | JF | 0.714 | 0.143 | 0.143 |
| 708 | 359.79357 | -11.53664 | JF | 0.500 | 0.214 | 0.286 |
| 712 | 359.95754 | -11.58909 | JF | 0.900 | 0.100 | 0.000 |
| 713 | 359.95392 | -11.53194 | JF | 0.833 | 0.167 | 0.000 |
| 715 | 358.59328 | -11.38965 | PM | 0.250 | 0.583 | 0.167 |

**Table 1 continued from previous page**

| | | | | | | |
|---|---|---|---|---|---|---|
| 722 | 358.62056 | -11.30949 | JM | 0.333 | 0.333 | 0.333 |
| 724 | 358.57568 | -11.25034 | JF | 0.500 | 0.333 | 0.167 |
| 728 | 358.75295 | -11.40814 | JF | 0.929 | 0.071 | 0.000 |
| 729 | 358.81247 | -11.47520 | JF | 0.500 | 0.214 | 0.286 |
| 732 | 358.86595 | -11.44845 | JF | 0.500 | 0.500 | 0.000 |
| 733 | 358.84499 | -11.39690 | JF | 0.667 | 0.000 | 0.333 |
| 753 | 359.14656 | -11.11274 | JF | 0.429 | 0.143 | 0.429 |
| 754 | 359.42591 | -11.19957 | JF | 0.333 | 0.333 | 0.333 |
| 755 | 359.57791 | -11.44225 | JF | 0.667 | 0.000 | 0.333 |
| 758 | 359.86357 | -11.06018 | M | 0.000 | 0.857 | 0.143 |
| 764 | 359.95285 | -10.82104 | PM | 0.100 | 0.700 | 0.200 |
| 767 | 358.58176 | -10.43162 | M | 0.000 | 0.571 | 0.429 |
| 772 | 359.26739 | -10.42607 | JF | 0.857 | 0.000 | 0.143 |
| 774 | 359.47995 | -10.42052 | JM | 0.500 | 0.167 | 0.333 |
| 776 | 359.98098 | -10.45068 | M | 0.167 | 0.833 | 0.000 |
| 782 | 360.22305 | -11.89648 | JF | 0.5 | 0.0 | 0.5 |
| 784 | 360.19973 | -11.70127 | M | 0.25 | 0.42 | 0.33 |
| 785 | 360.34671 | -11.72702 | M | 0.08 | 0.92 | 0.000 |
| 786 | 360.34486 | -11.72640 | M | 0.08 | 0.92 | 0.000 |
| 788 | 360.22373 | -11.67400 | JF | 0.666 | 0.167 | 0.167 |
| 801 | 360.29870 | -11.28749 | JF | 0.58 | 0.42 | 0.000 |
| 804 | 360.20985 | -11.26370 | M | 0.000 | 0.83 | 0.17 |
| 805 | 360.14277 | -11.09888 | M | 0.167 | 0.833 | 0.000 |
| 808 | 360.30438 | -11.10356 | JM | 0.500 | 0.500 | 0.000 |
| 809 | 360.01918 | -10.97637 | M | 0.08 | 0.587 | 0.333 |
| 810 | 360.21190 | -10.99979 | JF | 0.58 | 0.25 | 0.17 |
| 813 | 360.19632 | -10.80247 | JF | 0.5 | 0.333 | 0.17 |
| 814 | 360.21701 | -10.58690 | JF | 0.666 | 0.167 | 0.167 |
| 818 | 360.170991 | -10.42114 | JF | 0.67 | 0.000 | 0.33 |
| 822 | 360.27655 | -10.40025 | JF | 0.58 | 0.25 | 0.17 |
| 824 | 360.08211 | -9.69515 | JF | 0.666 | 0.167 | 0.167 |
| 826 | 360.08038 | -9.63207 | JF | 0.75 | 0.08 | 0.17 |
| 827 | 360.18443 | -9.56484 | JM | 0.167 | 0.666 | 0.167 |
| 829 | 360.21754 | -9.53093 | JF | 0.5 | 0.17 | 0.33 |
| 840 | 360.01387 | -10.72107 | JF | 0.5 | 0.0 | 0.5 |
| 842 | 360.18664 | -10.40580 | JF | 0.833 | 0.167 | 0.000 |
| 843 | 360.32517 | -10.42615 | JF | 0.67 | 0.000 | 0.33 |
